# Supplementary material for: Can Domains Be Transferred Across Languages in Multi-Domain Multilingual Neural Machine Translation?
Source: arXiv:2210.11628 source file (2022-10-20)
Supplement: Supplementary file 1 [file appendix.tex]

\section{Fusion adapter approach}

Our strategy is to learn a domain-agnostic encoder via domain discriminator and domain-specific decoder with domain-specific adapter layers(~\cref{fig:mdml-nmt}).

\COMMENT{COMMENT: Is it the proposed method? Or we are going to get this conclusion from our experiments?}

\begin{figure*}[]
    \centerline{\includegraphics[scale=0.55]{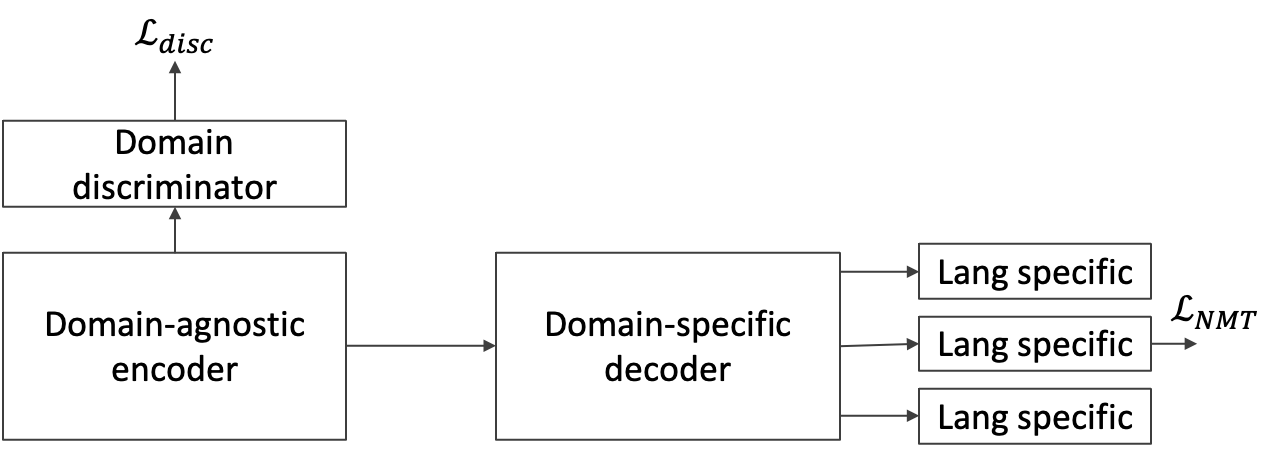}}
    \caption{Our proposed multi-domain multilingual NMT approach.}
    \label{fig:mdml-nmt}
\end{figure*}

\subsection{Domain-agnostic encoder}
Let $\textbf{h} = \textrm{enc}_\theta(x)$
be the representation of sentence $x$ computed by the mean-pooled average of the top layer's states of the NMT's encoder where $\theta$ is the parameters of NMT model.

$$
\mathcal{L}_{\textrm{disc}}(\theta, \psi) = -\log \Pr(d|\textbf{h};\psi) + \lambda \textrm{H}(\Pr(d|\textbf{h};\psi)
$$
where $\textrm{H}(\Pr(d|\textbf{h};\psi)$ is the entropy of
the probability distribution of the domain discriminator with N domain labels; $\psi$ is the parameters of the domain discriminator.

\subsection{Domain specific decoder}
We insert small adapter module in transformer layers of decoder. The adapter module includes a down-projection $\vW^{(l)}_{down}$ followed by a up-projection $\vW^{(l)}_{up}$ to project the hidden state $\vh^{(l)}$ in layer $l$ to a lower-dimension space then project back to high-dimension space (~\cref{fig:adapter})
\begin{align}
    \vh^{(l)} = \vh^{(l)} + f(\vh^{(l)}\vW^{(l)}_{down})\vW^{(l)}_{up}
\end{align}
where $f(.)$ is a nonlinear activation function.

We learn the adapter sublayer while freezing the share encoder and decoder parameters. At training time, we only train the adapter with the training data corresponding to a specific domain data. 

We hypothesise that the adapter layer allow to zero-shot transfer to unseen translation direction.

\subsection{Language specific adapter layer}
Language specific adapter is a transformer layer on top of decoder specialising on generate translation of a language group.

Or can we just append the target tags to the end of source sentences.

\section{Domain generalisation}
We aim to generalise the NMT model to unseen domains by  introduce the latent domain specific variable $\vz^l$ to decoder transformer layer $l$ and learn to combine the adapter layers of known domains. Given a sentence $\vx$ in source language and its translation $\vy$ in target language, the translation probability can be factorized as
\begin{align}
    \Pr(\vy|\vx;\theta) &= \prod_i\Pr(y_i|y_{<i},\vx;\theta) \\
    \Pr(y_i|y_{<i},\vx;\theta) &= \Pr(y_i|y_{<i},\vx,\vz_i;\theta)\Pr(\vz_i|y_{<i},\vx;\theta) \\
    \Pr(\vz_i|y_{<i},\vx;\theta) &= \prod_l^L\Pr(z_i^l|z_i^{<l},y_{<i},\vx;\theta)
\end{align}
where $z_i^l$ is the latent variable at layer $l$, position $i$, corresponding to the domain from which input sentence $\vx$ is generated from, $\theta$ is model parameters.

\begin{figure}[]
    \centerline{\includegraphics[scale=0.55]{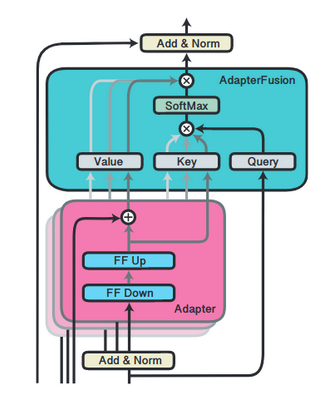}}
    \caption{Adapter with fusion layer.}
    \label{fig:adapter}
\end{figure}

After training the adapter sublayers, we learn the conditional domain likelihood $\Pr(\vz_i|\vx;\theta)$ with a fusion layer on top of adapter sublayers  while freezing all other parameters. Training data from all domain are fed to all adaptive sublayers and the fusion layer learned to combine their outputs. Assume that we have $K$ domain adapter sublayers, the translation probability can be computed as

% \begin{align}
%     \Pr(\vy|\vx;\theta) &= \prod\Pr(y_i|y_{<i,\vx;\theta}) \\
%     \Pr(y_i|y_{<i},\vx;\theta) &= \sum_{k^{(L)}}^{K} \Pr(\vz_{i,k^{(L)}|y_{<i},\vx;\theta)\Pr(y_i|y_{<i},\vx,\vz_i;\theta) \\
%     \Pr(\vz_i|y_{<i},\vx;\theta) &= \prod_l^L\Pr(z_i^l|z_i^{<l},y_{<i},\vx;\theta)
% \end{align}

In summary,
\begin{align}
    \Pr(\vy|\vx;\theta) &= \prod_i\Pr(y_i|y_{<i},\vx,\vz_i;\theta) \\
    &\times \prod_l^L\sum_{k^{(l)}}\Pr(z_{i,k^{(l)}}|\vx,z_i^{<l};\theta) 
\end{align}

\section{Training procedure}
\paragraph{Learn domain-agnostic NMT}. We first learn a domain agnostic NMT by training the NMT model with domain discriminator and language specific layers, but without the domain-specific adapter sublayers. The learning objective is
$$
\mathcal{L} = \mathcal{L}_{\textrm{disc}}(\theta, \psi) + \mathcal{L}_{\textrm{NMT}}(\theta)
$$
We add domain tag at the decoder side, and randomly replace the actual domain tag with \textsc{OOD} tag so that the NMT model can learn to handle the unseen domain tag.
\paragraph{Learn domain-specific adaptive sublayers.}
We add adapter sublayer into the trained domain-agnostic NMT in previous step. We freeze the encoder, decoder and only learn the adapter sublayers. Each sublayer is corresponding to a single domain. The training objective is
\begin{align}
\mathcal{L} &= - \sum_{(\vx,\vy)\in \mathcal{D}} \log \Pr(\vy_i|\vx_i;\theta)    \\
&= - \sum_{(\vx,\vy)\in \mathcal{D}} \sum_{\vz} \delta_{d(\vx_i), \vz_j}  \log  \Pr(\vy_i|\vx_i,\vz_j;\theta)
\end{align}
where $\delta_{d(\vx_i), \vz_j}$ is the Kronecker delta function  which is 1 if the domain $d(\vx_i)$ of the sentence $\vx_i$ is $j$ and 0 otherwise.

\paragraph{Learn domain-specific adapter fusion.} We train the fusion layers while freezing all other parameters. Training data from all domain are fed to all adaptive sublayers and the fusion layer learned to combine their outputs. We randomly treat some training inputs as unseen domain data. 

We aim to minimize the upperbound of the negative log likelihood of the translation $y$ condition on the input $x$
\begin{align}
&\min - \sum_{(\vx,\vy)\in \mathcal{D}} \log  \Pr(\vy_i|\vx_i;\theta) \leq \\
 &\min -\sum_{(\vx,\vy) \in \mathcal{D}} \sum_{\vz} \Pr(\vz_j|\vx_i;\theta) \log \Pr(\vy_i, \vz_j|\vx_i;\theta)
\end{align}

We also apply posterior regularisation to enforce the posterior probability $\Pr(\vz_j|\vx_i;\theta)$ to be close to true domain distribution for known domains, or to be close to uniform distribution for unseen domains. That is 
$$\textrm{KL}[\Pr(\vz|\vx_i;\theta)\parallel Q(\vz)]$$
where $Q(\vz_j) \sim \mathcal{U}(0,1)$ for unseen domains, and $Q(\vz_j)$ is soft-label encoding $\Tilde{e}_j$ for known domains $j$. With a small value $\epsilon \ll 1$, we define the sotf-label encoding $\Tilde{e}_j$ as follow, 
\begin{align}
    \Tilde{e}_j = (1-\epsilon)e_j + \frac{\epsilon}{n_d}
\end{align}
where $e_j$ is the one-hot vector for domain $j$, $n_d$ is number of domains. 

In summary, the objective function is
\begin{align}
  \mathcal{L} =  -&\sum_{(\vx,\vy) \in \mathcal{D}} \sum_{\vz} \Pr(\vz_j|\vx_i;\theta) \log \Pr(\vy_i, \vz_j|\vx_i;\theta) \\
  +& \textrm{KL}[\Pr(\vz|\vx_i;\theta)\parallel Q(\vz)]
\end{align}

% \begin{align}
%   \mathcal{L} =  -&\sum_{(\vx,\vy) \in \mathcal{D}}  \log \Pr(\vy_i, \vz_j|\vx_i;\theta) \\
%   +& \sum_{l}\sum_{\vz^{(l)}} \Pr(\vz^{(l)}_j|\vx_i;\theta) \\
%   +& \textrm{KL}[\Pr(\vz|\vx_i;\theta)\parallel Q(\vz)]
% \end{align}
